# Supplementary material for: SwiFT: Swin 4D fMRI Transformer
Source: arXiv:2307.05916 source file (2023-10-31)
Supplement: Supplementary file 1 [file table1.tex]

\begin{table}
\caption{
Efficiency comparison of different position embedding methods
% \textbf{.}
% 
} % \caption
\centering

\resizebox{\linewidth}{!}{ %< auto-adjusts font size to fill line
\begin{tabular}{lllllll}

\toprule
\multicolumn{1}{c}{\multirow{1}{*}{Method}} &
  \multicolumn{1}{c}{\# param.} &
  \multicolumn{1}{c}{FLOPs} &
  \multicolumn{1}{c}{throughput} \\
  \midrule
% SwiFT-rel (HCP)   & 2.059M & 1.73G  &  103.84  \\ 
% SwiFT-abs (HCP)   & 1.971M & 1.73G  &   117.61 \\
% SwiFT-rel (ABCD)   & 4.668M & 2.62G  &   94.17  \\ 
% SwiFT-abs (ABCD)   & 4.649M & 2.62G  &   104.46  \\ 
SwiFT-rel (HCP)   & 2.05M & 1.73G  &  103.84  \\ 
SwiFT-abs (HCP)   & 1.97M & 1.73G  &   117.61 \\
SwiFT-rel (ABCD)   & 4.66M & 2.62G  &   94.17  \\ 
SwiFT-abs (ABCD)   & 4.64M & 2.62G  &   104.46  \\
\bottomrule
\end{tabular}} %\resizebox
\label{tab:result3}
\end{table}
